# Supplementary material for: Communication-Efficient Collaborative Perception via Information Filling with Codebook
Source: arXiv:2405.04966 source file (2024-05-08)
Supplement: Supplementary file 1 [file 7_suppl.tex]

\clearpage
\setcounter{page}{1}
\maketitlesupplementary

% \section{Rationale}
% \label{sec:rationale}
% % 
% Having the supplementary compiled together with the main paper means that:
% % 
% \begin{itemize}
% \item The supplementary can back-reference sections of the main paper, for example, we can refer to \cref{sec:intro};
% \item The main paper can forward reference sub-sections within the supplementary explicitly (e.g. referring to a particular experiment); 
% \item When submitted to arXiv, the supplementary will already included at the end of the paper.
% \end{itemize}
% % 
% To split the supplementary pages from the main paper, you can use \href{https://support.apple.com/en-ca/guide/preview/prvw11793/mac#:~:text=Delete%20a%20page%20from%20a,or%20choose%20Edit%20%3E%20Delete).}{Preview (on macOS)}, \href{https://www.adobe.com/acrobat/how-to/delete-pages-from-pdf.html#:~:text=Choose%20%E2%80%9CTools%E2%80%9D%20%3E%20%E2%80%9COrganize,or%20pages%20from%20the%20file.}{Adobe Acrobat} (on all OSs), as well as \href{https://superuser.com/questions/517986/is-it-possible-to-delete-some-pages-of-a-pdf-document}{command line tools}.

Here, we start with module design details and give out more implementation details, then introduce the dataset details, including generation and qualitative samples, and the exact values for the benchmarks.

\section{Detailed Information About Module Designs}
\subsection{Information-filling-driven message selection}

\noindent\textbf{Solution.} Alg.~\ref{alg:selection} presents the solution of our information-filling-driven message selection, this is, 
\vspace{-2mm}
\begin{footnotesize}
\begin{subequations}
    \begin{align}
        &\{ \mathbf{M}_{i \rightarrow j}^{*} \}_{i,j} \ = \ \underset{\mathbf{M}}{\rm argmax}\sum_{j=1}^{N} f_{\rm min}\left(\mathbf{C}_j+\sum_{i=1,i\neq j}^{N}\mathbf{M}_{i\rightarrow j}\odot \mathbf{C}_{i},u\right),\label{eq:selector}\\
        &{\rm where}\sum_{i,j=1,j\neq i}^{N}\mathbf{M}_{i\rightarrow j} \leq b,\mathbf{M}_{i\rightarrow j}\in\{0,1\}^{H\times W}\label{eq:constraint}.
    \end{align}
\end{subequations}    
\end{footnotesize}Here, $\mathbf{M}_{i\rightarrow j} \in \{0,1\}^{H \times W}$ is the binary selection matrix supported on the BEV map. Each element in the matrix indicates whether Agent $i$ should send the information to Agent $j$ at a specific spatial location (1 for sending information, and 0 for not sending). $\odot$ denotes element-wise multiplication, and the scalar $u$ is a hyper-parameter to reflect the upper bound of information demand. 
The function $f_{\rm min}(\cdot,\cdot)$ computes the element-wise minimum between a matrix and a scalar.

Despite the hard constraints and non-differentiability of binary variables in this proxy-constrained optimization problem, it possesses an analytical solution. We tackle this by splitting the optimization into two sub-problems: i) optimizing the maximization in Equation~\eqref{eq:selector} without the constraint in Equation~\eqref{eq:constraint} and removing the indifferentiable thresholding function $f_{\rm min}(\cdot)$; ii) addressing the equivalent maximization problem of Equation~\eqref{eq:selector} while considering the constraint in Equation~\eqref{eq:constraint}.

$\bullet$ The first sub-problem involves unconstrained maximization optimization, which is given by
\begin{footnotesize}
\begin{subequations}
\begin{align}
        &\{ \overline{\mathbf{M}}_{i \rightarrow j}\}_{i,j} \ = \ \underset{\mathbf{M}}{\rm argmax}\sum_{j=1}^{N} f_{\rm min}\left(\mathbf{C}_j+\sum_{i=1,i\neq j}^{N}\mathbf{M}_{i\rightarrow j}\odot \mathbf{C}_{i},u\right),\label{eq:selector_thre}\\
        &{\rm where}~\mathbf{M}_{i\rightarrow j}\in\{0,1\}^{H\times W}.\label{eq:constraint_thre}
    \end{align}
\end{subequations}    
\end{footnotesize}This involves selecting the highest-scoring regions to meet the information demand, excluding unnecessary information for each sender-receiver pair, resulting in $\overline{\mathbf{M}}_{i \rightarrow j}$. Steps include:
a) Sorting scores from all collaborators in descending order for each spatial location;
b) Accumulating these scores until reaching the information demand threshold and disregarding the rest, refining the subset.

By doing so, we can remove the indiscernible cutoff by using the optimized matrix $\overline{\mathbf{M}}_{i \rightarrow j}$ to focus on required information scores, this is,
\begin{footnotesize}
\begin{subequations}
\begin{align}
    f_{\rm min}\left(\mathbf{C}_j+\sum_{i=1,i\neq j}^{N}\mathbf{M}_{i\rightarrow j}\odot \mathbf{C}_{i},u\right)&=\mathbf{C}_{j}+\overline{\mathbf{M}}_{i\rightarrow j}\odot \mathbf{C}_{i},\\
    &=\mathbf{C}_{j}+\mathbf{C}_{i\rightarrow j}.\label{eq:cutoff}
\end{align}
\end{subequations} 
\end{footnotesize}

$\bullet$ The second sub-problem is a proxy-constrained maximization optimization without an indiscernible cutoff. By substituting Equation~\eqref{eq:cutoff} into  Equation~\eqref{eq:selector}, we get an equivalent formulation of the original optimization in Equation~\eqref{eq:selector},
\begin{subequations}
    \begin{align}
        &\{ \mathbf{M}_{i \rightarrow j}^{*} \}_{i,j} \ = \ \underset{\mathbf{M}}{\rm argmax}\sum_{j=1}^{N} \sum_{i=1,i\neq j}^{N}\mathbf{M}_{i\rightarrow j}\odot \mathbf{C}_{i\rightarrow j},\label{eq:selector_nothre}\\
        &{\rm where}\sum_{i,j=1,j\neq i}^{N}\mathbf{M}_{i\rightarrow j} \leq b,\mathbf{M}_{i\rightarrow j}\in\{0,1\}^{H\times W}\label{eq:constraint_nothre}.
    \end{align}
\end{subequations} 
This optimization has an analytical solution, which involves selecting top-$b$ ranked spatial regions based on elements in $\mathbf{M}$. The steps are:
c) Resorting all retained scores across spatial regions in descending order; 
d) Forming $\mathbf{M}^{*}$ by marking top-$b$ elements in this list as $1$, others as $0$. 

Note that, information demand is fulfilled in b), communication constraint is met in d), and maximization is achieved through prioritization in a) and c). Collectively, these steps yield an optimal solution for the constrained optimization problem in Equation~\eqref{eq:selector} and Equation~\eqref{eq:constraint}.

% ; and ii) even we cannot solve the original objective, this proxy objective still carries the similar idea to promote better, yet more compact perception.

\noindent\textbf{Computation cost.} Step c is the most computationally demanding, involving the sorting of all necessary spatial regions to meet the information demand. However, in our scenario, the precise order is irrelevant; we only need to identify the top-$b$ elements from $m$ spatial region candidates, resulting in a computational cost of $O(\log(m))$. By concentrating on the highly sparse foreground areas, we significantly lower this cost to a negligible level, thus allowing each agent to offer more focused support to others at minimal expense.

\begin{algorithm*}[!htbp]
\caption{Information-filling-driven Message Selection}\label{alg:selection}
\begin{algorithmic}[1]
\Require Spatial information score maps $\{\mathbf{C}_i\}_{i=1}^{N}$ of $N$ agents with dimensions $(H,W)$, information demand $u$, communication budget $b$.
\Ensure Selection matrices $\{\mathbf{M}_{i \rightarrow j}\}_{j=1,j\neq i}^{N}$ for each agent pair $(i, j)$.
\State {\color{blue} { \#~Select the required information to fulfill the receiver's information demand from high-scoring senders per-location}}
\State {\color{blue} { \#~Initialization}}
\ForAll{$i \in \{1, \ldots, N\}, j \in \{1, \ldots, N\}$}
    \State $\overline{\mathbf{M}}_{i \rightarrow j} = \mathbf{0}\in\{0,1\}^{H\times W}$ 
\EndFor
% \For{each location $(h,w)$ within the spatial map}
\ForAll{$j \in \{1, \ldots, N\}$}  \Comment{Receiver}
\For{$h \in \{0, \ldots, H-1\}, w \in \{0, \ldots, W-1\}$} \Comment{Per-location}
    \State {\color{blue} { \#~\textbf{Step a: Prioritize senders with higher scores}}}
    \State $R = f_{\rm rank}(\{\mathbf{C}_i[h,w]\}_{i=1,i\neq j}^{N})$ \Comment{Senders}
    \State $s = \mathbf{C}_j[h,w]$ \Comment{The receiver's initial information amount}
    \State {\color{blue} { \#~\textbf{Step b: Exclude information over information demand}}}
    \State $A = []$ \Comment{The selected senders per-location}
    \For{each $\mathbf{C}_i[h,w]$ in $R$}
        \If{$s \leq u$} \Comment{Check the whether the information demand is reached}
            \State {\color{blue} { \#~Select sender}}
            \State $s = s + \mathbf{C}_i[h,w]$
            \State Append $i$ to $A$
        \Else
            \State {\color{blue} { \#~Stop selection once demand is met}}
            \State \textbf{break}
        \EndIf
    \EndFor
    \State {\color{blue} { \#~Select the required regions whose accumulated information below information demand}}
    \ForAll{$i \in A$}
        \State $\overline{\mathbf{M}}_{i \rightarrow j}[h,w] = 1$
    \EndFor
\EndFor
\State {\color{blue} { \#~Exclude information over demand}}
\ForAll{$i \in \{1, \ldots, N\} \setminus \{j\}$}
    \State $\mathbf{C}_{i\rightarrow j} = \mathbf{C}_i \odot \overline{\mathbf{M}}_{i \rightarrow j}$ 
\EndFor
\EndFor
\State {\color{blue} { \#~Select the most beneficial information within the communication budget among all the needed spatial regions}}
\State {\color{blue} { \#~Initialization}}
\ForAll{$i \in \{1, \ldots, N\}, j \in \{1, \ldots, N\}$}
    \State $\mathbf{M}_{i \rightarrow j} = \mathbf{0}\in\{0,1\}^{H\times W}$ 
\EndFor
\State {\color{blue} { \#~\textbf{Step c: Prioritize information with higher scores}}}
\State $R \gets f_{\rm rank}(\{\mathbf{C}_{i\rightarrow j}\}_{i,j=1,i\neq j}^{N})$ \Comment{All the required spatial regions between all the sender-receiver pairs}
\State {\color{blue} { \#~\textbf{Step d: Exclude information over communication budget}}}
\ForAll{$j \in \{1, \ldots, N\}$}  \Comment{Receiver}
\ForAll{$i \in \{1, \ldots, N\} \setminus \{j\}$}   \Comment{Sender}
    \For{$h \in \{0, \ldots, H-1\}, w \in \{0, \ldots, W-1\}$}  \Comment{Per-location}
        \If{$\mathbf{C}_{i\rightarrow j}[h,w]$ is in top-$b$ of $R$}
            \State $\mathbf{M}_{i \rightarrow j}[h, w] = 1$
        \EndIf
    \EndFor
\EndFor
\EndFor
\State \textbf{return} $\{\mathbf{M}_{j \rightarrow i}\}_{i,j=1,i\neq j}^{N}$
\end{algorithmic}
\end{algorithm*}

\subsection{Codebook-based message representation}

\noindent\textbf{Extensibility for new heterogeneous agents.} The codebook representation creates a common feature space that enables the integration of new heterogeneous agents. In the training phase, perceptual features from all agents, whether equipped with camera or LiDAR sensors, are collected in $\digamma$ for codebook training. This process benefits from joint supervision using diverse inputs, enhancing learning efficiency and ensuring that critical perceptual information is retained. As a result, the optimized task-adaptive codebook $\mathbf{D}^*$ encapsulates the essential features from various modalities. During inference, all agents utilize this optimal codebook $\mathbf{D}^*$ directly.

\noindent\textbf{Adaptability for codebook configuration.} The codebook's configuration is highly adaptable, allowing for adjustments in both the size of the codebook $n_L$ and the number of codes $n_R$ utilized for representing the input vector. During training, we vary the code quantity from $1$ to $n_R$, enabling the optimized codebook to accommodate different configurations and communication budgets during inference.

During training, especially with an increased number of codes, the representation comprises combinations of multiple codes. Consequently, task-driven codebook learning entails the aggregation of these codes for feature approximation at each spatial location. This process is defined as follows,
\begin{small}
\begin{subequations}
\begin{align}
\label{eq:codebook_learning_multiple}
\mathbf{D}^*&= \arg\min_{\mathbf{D}} \sum_{\mathcal{F}\in\digamma}
\sum_{h,w} \min_{\{\ell_r\}_{r=1}^{n_R}} \left( \Psi( \mathbf{F}_d ) + \left\| \mathcal{F}_{[h,w]} - \mathbf{F}_d \right\|_2^2 \right),\\
&{\rm where}~~\mathbf{F}_d=\sum_{\ell_r\in \mathcal{L}_{n_R}}\mathbf{D}_{[\ell_r]},\mathcal{L}_{n_R}=\{\ell_r\}_{r=1}^{n_R}.
\end{align}
\end{subequations}
\end{small}Here, $\mathbf{F}_d$ is a combination of codes $\{\mathbf{D}_{[\ell_r]}\}_{r=1}^{n_R}$, and $\Psi(\cdot)$ measures the detection performance achieved by replacing $\mathcal{F}_{[h,w]}$ with $\mathbf{F}_d$. The code index set $\mathcal{L}_{n_R}=\{\ell_r\}_{r=1}^{n_R}$ is selected to minimize the reconstruction error in a greedy way. As $n_r$ ranges from $1$ to $n_R$, the optimization of the code index is carried out as follows
\begin{small}
\begin{equation}
\label{eq:codeindex_optimization}
l_r^{*}= \min_{\mathcal{L}_{n_{r-1}} \cup \{l_r\}} \left\| \mathcal{F}_{[h,w]} - \sum_{\ell_k\in \mathcal{L}_{n_{r-1}}\cup \{l_r\}}\mathbf{D}_{[\ell_k]} \right\|_2^2.
\end{equation}
\end{small}In this process, the code index $l_r^{*}$ is determined by minimizing the reconstruction error, which is the L2 norm of the difference between the feature vector $\mathcal{F}_{[h,w]}$ and the sum of the selected codes from the codebook $\mathbf{D}$. The selection at each step involves the union of the set $\mathcal{L}_{n_{r-1}}$, representing the previously selected indices, and the new index $l_r^{*}$.

During inference, each agent leverages the optimized codebook $\mathbf{D}$ to convert the selected sparse feature map $\mathcal{Z}_{i\rightarrow j}$ into code indices $\mathcal{I}_{i\rightarrow j}$. At each Bird's Eye View (BEV) location $(h,w)$, given a code quantity of $n_r$, the code index is obtained as follows,
\vspace{-1mm}
\begin{small}
\begin{eqnarray}
\label{eq:code_index}
{(\mathcal{I}_{i\rightarrow j})}_{[h,w]} = \arg \min_{\mathcal{L}_{n_{r}}} \left\| {(\mathcal{Z}_{i\rightarrow j})}_{[h,w]} - \sum_{\ell_k\in \mathcal{L}_{n_{r}}}\mathbf{D}_{[\ell_k]}\right\|_2^2.
\end{eqnarray}    
\end{small}This method aligns with Equation~\eqref{eq:codeindex_optimization} to create the optimized set of code indices $\mathcal{L}_{n_r}=\{\ell_k\}_{k=1}^{n_r}$. The value of $n_r$, ranging from $1$ to $n_R$, allows the codebook to be flexible for different configurations and communication requirements during deployment.

\section{Additional Experimental Results}

\subsection{Robustness assessment under more metrics}

\begin{figure*}[!t]
\vspace{-1mm}
\begin{minipage}{.49\linewidth}
  \centering
  % \begin{subfigure}{0.48\linewidth}
  %   \includegraphics[width=0.9\linewidth]{Figs/Robust_PoseError/OPV2V_LiDAR_AP50.png}
  %   \caption{OPV2VH+}
  % \end{subfigure}
  % \begin{subfigure}{0.48\linewidth}
  %   \includegraphics[width=0.9\linewidth]{Figs/Robust_PoseError/DAIRV2X_LiDAR_AP50.png}
  %   \caption{DAIR-V2X}
  % \end{subfigure}
  \begin{subfigure}{0.98\linewidth}
    \includegraphics[width=1.0\linewidth]{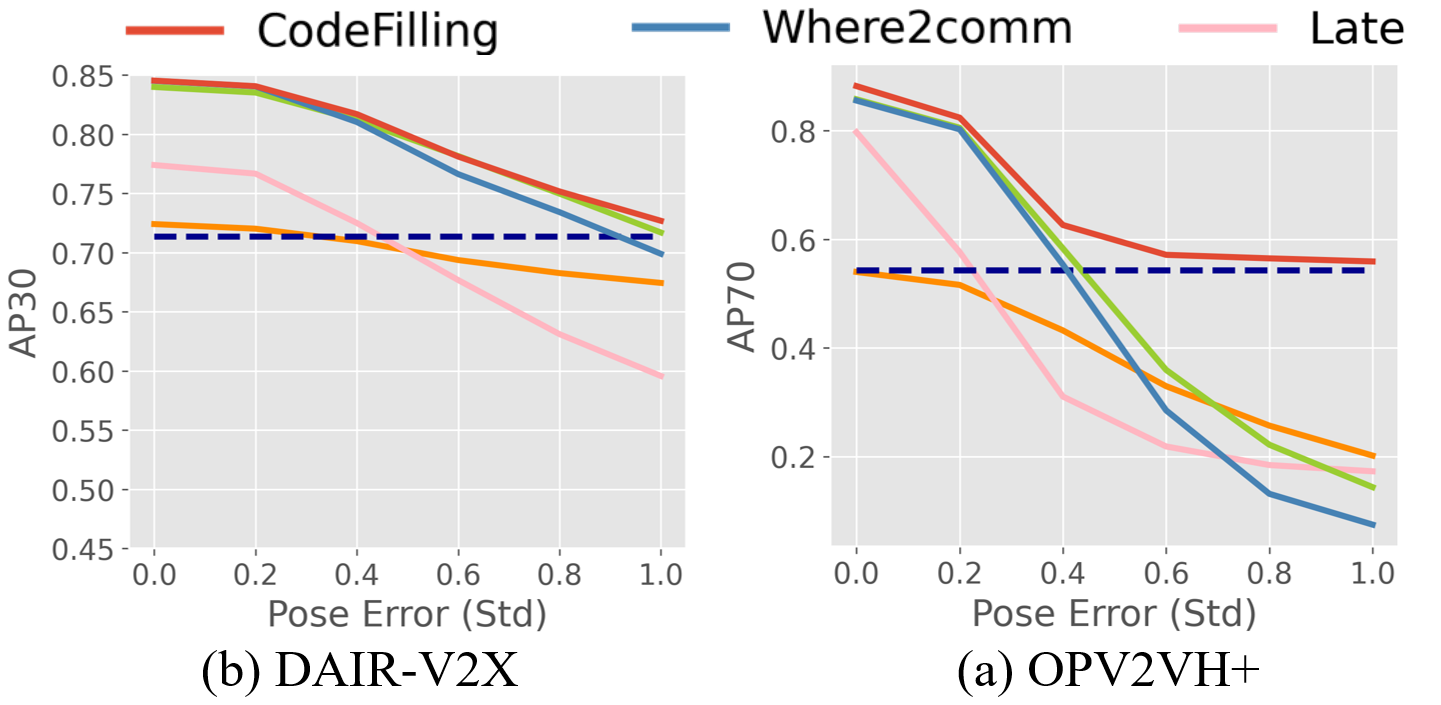}
  \end{subfigure}
  \vspace{-3mm}
  \caption{\texttt{CodeFilling} is robust to pose error issue.}
  \vspace{-3mm}
  \label{Fig:Robust_poseerror_AP3070}
\end{minipage}
\begin{minipage}{.49\linewidth}
  \centering
  % \begin{subfigure}{0.48\linewidth}
  %   \includegraphics[width=0.9\linewidth]{Figs/Robust_Latency/OPV2V_LiDAR_AP50.png}
  %   \caption{OPV2VH+}
  % \end{subfigure}
  % \begin{subfigure}{0.48\linewidth}
  %   \includegraphics[width=0.9\linewidth]{Figs/Robust_Latency/DAIRV2X_LiDAR_AP50.png}
  %   \caption{DAIR-V2X}
  % \end{subfigure}
   \begin{subfigure}{0.98\linewidth}
    \includegraphics[width=1.0\linewidth]{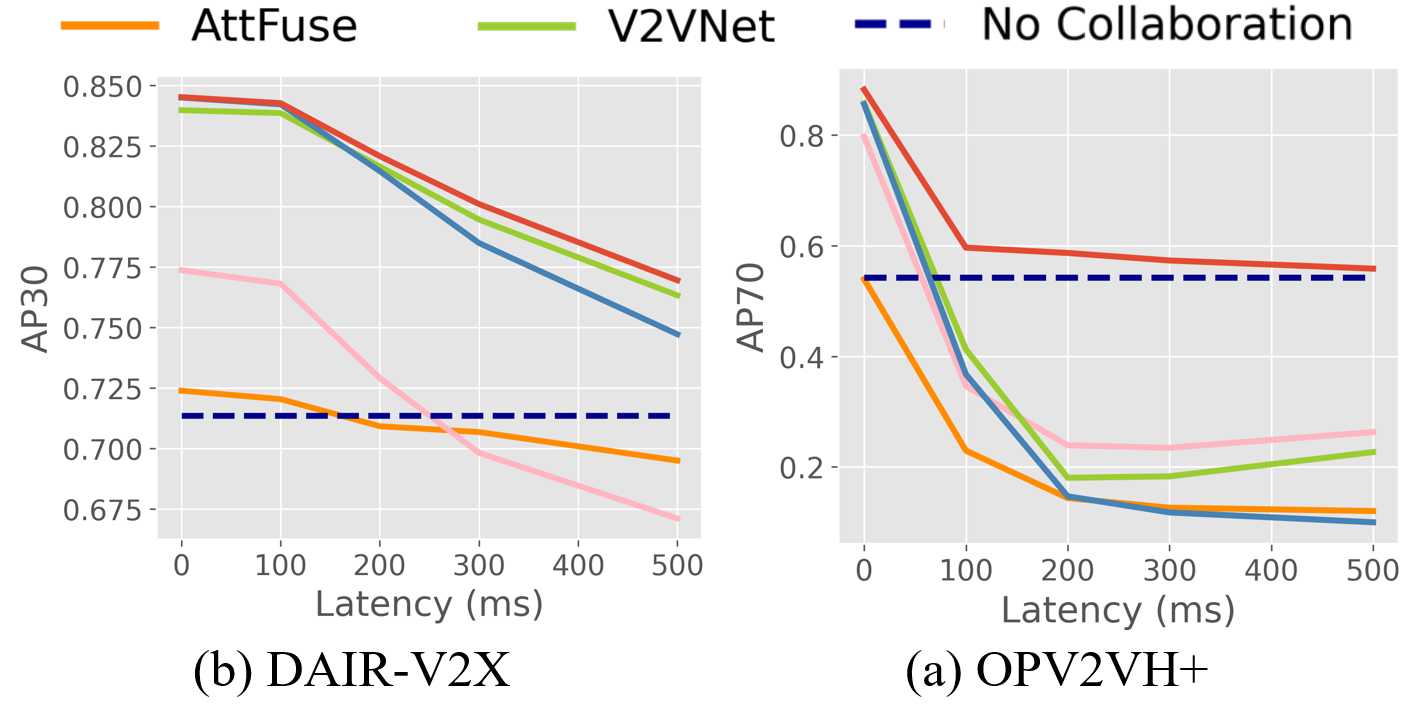}
  \end{subfigure}
  \vspace{-3mm}
  \caption{\texttt{CodeFilling} is robust to communication latency issue.} 
  % \Note{sc: left dairv2x, right opv2v}}
  \vspace{-3mm}
  \label{Fig:Robust_latency_AP3070}
  \end{minipage}
\end{figure*}

We validate the robustness against pose error and communication latency on both OPV2VH+ and DAIR-V2X under camera-only and heterogeneous settings. The pose error setting follows CoAlign~\cite{LuRobust:ICRA23} using Gaussian noise with a mean of 0m and standard deviations ranging from 0m to 1.0m. The latency setting follows SyncNet~\cite{LeiLatency:ECCV22}, varying from 0ms to 500ms. Figs.~\ref{Fig:Robust_poseerror_AP3070} and~\ref{Fig:Robust_latency_AP3070} show the detection performances as a function of pose error and latency, respectively in terms of AP30 and AP70. We see: i) while perception performance generally declines with increasing levels of pose error and latency, \texttt{CodeFilling} consistently outperforms baselines under all imperfect conditions; ii) \texttt{CodeFilling} consistently surpasses No Collaboration, whereas baselines fail when pose error exceeds 0.4m and latency surpasses 100ms. In \texttt{CodeFilling}, setting a lower information demand $u$ in situations with pose errors and latency issues allows each agent to collect less misleading collaborative information, thereby at least maintaining their individual performance.

\subsection{Discussion on the realistic limitations}
There are many challenges in a collaborative perception system. In this work, we focus on the bottleneck challenge in current collaborative perception systems; that is, the trade-off between communication bandwidth and perception performance. This challenge has been actively addressed in previous works~\cite{LiuWho2com:ICRA20,LiuWhen2com:CVPR20,HuWhere2comm:NeurIPS22,HuCollaboration:CVPR23}. Collaborative perception is enabled and also severely limited by the communication capacity, which is critically reflected in the highly dynamic and limited bandwidth in real-world communication systems. \texttt{CodeFilling} flexibly adapts to various communication bandwidths, achieving superior performance-bandwidth trade-off.

Here we further discuss other realistic limitations, assess the robustness of our system, and future improvements to be made. 

$\bullet$ For other realistic communication issues such as \textbf{latency}, \textbf{time synchronization}, \textbf{pose error}, \textbf{attack}, \texttt{CodeFilling} communicates strategically when necessary, rather than all the time or everywhere, to reduce the possibility of encountering communication problems. And \texttt{CodeFilling} can set a lower information demand $u$ in situations with these issues, which allows each agent to collect less misleading collaborative information, thereby at least maintaining their individual performance.

$\bullet$ For the \textbf{data availability}, \texttt{CodeFilling} works on both RGB and point cloud modalities and is sensor-friendly, so it can be deployed on cheap camera sensors and lidar sensors. And it accommodates heterogeneous settings where agents with different equipment can also collaborate with each other.

% \subsection{Ablation on codebook}

% \begin{itemize}
%     \item detection results fused and decoded from the last codebook compressor
%     \item detection results fused and decoded from every codebook compressor
% \end{itemize}

% \noindent\textbf{Statistical analysis of codebook features}

% 1 histogram or 1 table: error with origin feature/(?variance) within codebook -- different codebook configurations

% 1 scatter?: ap@xx -- error with origin feature (full comm)

% \subsection{Ablation on agent number}

% redundancy ratio -- agent number

\begin{table*}[!t]
\centering
\setlength\tabcolsep{2pt}
\caption{Overall performance on DAIR-V2X. The communication cost is denoted as $B$.}
\vspace{-3mm}
\centering
\begin{tabular}{l|cc|cc|cc}
\hline
Dataset      & \multicolumn{6}{c}{DAIR-V2X}                     \\ \hline
Setting      & \multicolumn{2}{c|}{LiDAR} & \multicolumn{2}{c|}{Camera} & \multicolumn{2}{c}{Heterogeneous} \\ \hline
Method/Metric         & $B$  & AP@30/50 & $B$  & AP@30/50 & $B$  & AP@30/50   \\ \hline
No Collaboration    & 0.00  & 71.35/67.27   & 0.00 & 5.65/1.93   & 0.00 & 5.54/1.92       \\
Late                & 19.43 & 77.40/69.54   & 19.43 & 15.82/6.59 & 19.43 & 40.82/25.14     \\
AttFuse             & 22.62 & 72.38/64.83   & 22.62 & 2.63/0.63  & 22.62 & 12.93/3.71      \\
DiscoNet            & 22.62 & 82.16/78.60   & 22.62 & 6.43/1.78  & 22.62 & 28.88/16.15     \\
V2VNet              & 22.62 & 83.98/79.28   & 22.62 & 19.81/7.38 & 22.62 & 47.14/28.47     \\
HMViT               & 22.62 & 77.09/69.92   & 22.62 & 6.65/1.40  & 22.62 & 39.78/20.83   \\ \hline
\multirow{5}{*}{Where2comm} 
& 0.00  & 71.35/67.27   & 0.00  &  5.65/1.93 & 0.00  &  5.54/ 1.92     \\
& 13.85 & 82.39/77.07   & 13.70 & 18.47/7.36 & 13.88 & 38.73/22.30     \\
& 14.94 & 83.73/78.48   & 15.59 & 19.59/7.86 & 14.95 & 43.39/26.29     \\
& 19.42 & 84.50/79.24   & 21.59 & 21.90/8.32 & 19.40 & 47.47/29.73     \\
& 22.62 & 84.50/79.39   & 22.62 & 21.96/8.34 & 22.62 & 47.47/30.00     \\\hline 
\multirow{7}{*}{\textbf{CodeFilling}} 
& 0.00  & 71.35/67.27   & 0.00  &  5.65/1.93 & 0.00  &  5.54/ 1.92    \\
& 4.96  & 79.80/75.60   & 4.88  & 15.30/6.03 & 5.00  & 33.83/19.19    \\
& 6.98  & 82.52/77.73   & 6.86  & 18.30/7.10 & 6.09  & 39.45/23.72    \\
& 8.09  & 84.00/79.39   & 8.68  & 19.63/7.83 & 8.11  & 42.61/25.43    \\
& 12.12 & 84.47/79.91   & 14.41 & 22.01/8.50 & 12.09 & 46.89/28.69    \\
& 15.62 & 84.52/79.99   & 15.62 & 22.22/8.51 & 15.62 & 47.51/29.14    \\
& 22.26 & \textbf{84.52}/\textbf{79.99}   & 22.26 & \textbf{22.22}/\textbf{8.51} & 22.26 & \textbf{47.51}/\textbf{30.00}   \\\hline 
\end{tabular}
\label{tab:SOTA_performance}
\vspace{-3mm}
\end{table*}

\begin{table*}[!t]
\centering
\setlength\tabcolsep{2pt}
\caption{Overall performance on OPV2VH+. The communication cost is denoted as $B$.}
\centering
\begin{tabular}{l|cc|cc|cc}
\hline
Dataset     & \multicolumn{6}{c}{OPV2VH+}                      \\ \hline
Setting     & \multicolumn{2}{c}{LiDAR} & \multicolumn{2}{c}{Camera} & \multicolumn{2}{c}{Heterogeneous} \\ \hline
Method/Metric     & $B$  & AP@50/70 & $B$  & AP@50/70 & $B$   & AP@50/70  \\ \hline
No Collaboration      & 0.00  & 68.83/54.27   & 0.00  & 15.43/4.97  & 0.00  & 44.20/30.57    \\
Late                  & 23.08 & 86.57/79.51   & 23.08 & 51.37/27.71 & 23.08 & 78.55/66.02     \\
AttFuse               & 26.27 & 76.55/53.95   & 26.27 & 28.08/10.18 & 26.27 & 63.21/43.51     \\
DiscoNet              & 26.27 & 80.13/61.15   & 26.27 & 35.16/12.42 & 26.27 & 67.59/47.17     \\
V2VNet                & 26.27 & 90.06/85.73   & 26.27 & 64.18/43.40 & 26.27 & 87.96/80.13     \\
HMViT                 & 26.27 & 89.55/80.79   & 26.27 & 57.05/26.19 & 26.27 & 86.89/71.61   \\ \hline
\multirow{5}{*}{Where2comm} 
& 0.00  & 68.54/54.04   & 0.00  & 15.29/ 4.92 & 0.00  & 43.75/30.27     \\
& 17.25 & 85.39/79.44   & 16.49 & 50.16/25.94 & 16.90 & 77.16/63.60     \\
& 18.77 & 89.71/85.14   & 18.57 & 58.99/38.75 & 18.66 & 85.33/78.39     \\
& 22.63 & 90.76/85.36   & 25.81 & 65.05/47.66 & 25.01 & 88.19/83.31     \\
& 26.27 & 90.77/85.53   & 26.27 & 67.28/48.90 & 26.27 & 88.42/79.63     \\\hline 
\multirow{7}{*}{\textbf{CodeFilling}} 
& 0.00  & 68.54/54.04   & 0.00  & 15.29/4.92  & 0.00  & 43.75/30.27     \\
& 8.10  & 85.65/75.14   & 6.26  & 35.40/13.69 & 6.41  & 65.15/46.61     \\
& 9.27  & 87.38/77.90   & 8.40  & 43.79/20.01 & 8.30  & 75.47/56.74     \\
& 13.22 & 89.90/85.79   & 12.29 & 55.11/31.59 & 12.21 & 82.90/71.88     \\
& 16.04 & 90.53/86.94   & 18.92 & 63.89/43.78 & 18.15 & 87.43/80.45     \\
& 19.51 & 90.66/86.99   & 19.51 & 66.39/47.77 & 19.51 & 88.05/80.98     \\
& 25.60 & \textbf{90.82}/\textbf{88.19}   & 25.61 & \textbf{67.39}/\textbf{51.16} & 25.61 & \textbf{88.58}/\textbf{83.65}     \\\hline 
\end{tabular}
\label{tab:SOTA_performance}
\vspace{-3mm}
\end{table*}

\begin{table*}[!t]
\centering
\setlength\tabcolsep{2pt}
\caption{Robustness to pose error on DAIR-V2X.}
\vspace{-3mm}
\begin{tabular}{l|ccccc}
\hline
Dataset   & \multicolumn{5}{c}{DAIR-V2X} \\ \hline
Method/Metric                              &  \multicolumn{5}{c}{AP30/AP50$\uparrow$}\\ \hline
Noise Level $\sigma_t/\sigma_r$($m/^{\circ}$)   & 0.0/0.0 & 0.2/0.2 & 0.4/0.4 & 0.6/0.6 & 1.0/1.0  \\ \hline
No Collaboration     & 71.35/67.27 & 71.35 /67.27 & 71.35 /67.27  & 71.35 /67.27  & 71.35 /67.27  \\
Late                 & 77.39/69.53 & 76.66 /67.04 & 72.49 /59.92  & 67.67 /54.89 & 59.57 /50.17 \\
AttFuse              & 72.40/64.87 & 72.01 /64.22 & 70.96 /62.89  & 69.36 /61.82  & 67.43 /60.98  \\
%DiscoNet             & 82.17/78.60 & 81.93 /77.65 & 80.68 /75.12  & 79.03 /72.76  & 75.74 /70.31    \\
V2VNet               & 83.98/79.28 & 83.51 /77.13 & 81.19 /71.88  & 75.15 /67.92  & 71.69 /62.74   \\
Where2comm           & 84.50/79.39 & 84.03 /77.12 & 81.02 /70.31  & 76.62 /64.92  & 69.89 /59.10  \\\hline 
\textbf{CodeFilling} & \textbf{84.52}/\textbf{79.99} & \textbf{84.05} /\textbf{78.05} & \textbf{81.69} /\textbf{72.58}  & \textbf{78.10} /\textbf{68.47}  & \textbf{72.68} /\textbf{67.99}  \\\hline 
\end{tabular}
\label{tab:Robustness_PoseError}
\vspace{-3mm}
\end{table*}

\begin{table*}[!t]
\centering
\setlength\tabcolsep{2pt}
\caption{Robustness to pose error on OPV2VH+.}
\vspace{-3mm}
\begin{tabular}{l|ccccc}
\hline
Dataset    &\multicolumn{5}{c}{OPV2VH+}  \\ \hline
Method/Metric    &\multicolumn{5}{c}{AP50/AP70$\uparrow$} \\ \hline
Noise Level $\sigma_t/\sigma_r$($m/^{\circ}$)   & 0.0/0.0 & 0.2/0.2& 0.4/0.4 & 0.6/0.6 & 1.0/1.0 \\ \hline
No Collaboration     & 68.83 /54.27  & 68.83 /54.27  & 68.83 /54.27  & 68.83 /54.27  & 68.83 /54.27   \\
Late                 & 86.86 /79.70  & 85.24 /57.63  & 63.86 /31.02  & 44.13 /21.83  & 28.90 /17.26  \\
AttFuse              & 76.56 /53.97  & 75.98 /51.58  & 72.95 /43.20  & 66.19 /32.93  & 49.08 /20.15  \\
%DiscoNet             & 80.13 /61.13  & 79.44 /59.09  & 76.82 /51.16  & 67.31 /37.06  & 43.09 /17.55  \\
V2VNet               & 90.06 /85.76  & 89.74 /80.52  & 86.24 /58.30  & 74.63 /35.93  & 44.59 /14.34  \\
Where2comm           & 90.77 /85.53  & 90.20 /80.23  & 83.33 /55.33  & 68.52 /28.48  & 29.07 /7.44  \\\hline 
\textbf{CodeFilling} & \textbf{90.82} /\textbf{88.19}  & \textbf{90.29} /\textbf{82.38}  & \textbf{84.23} /\textbf{62.61}  & \textbf{74.28} /\textbf{57.12}  & \textbf{72.53} /\textbf{55.90}  \\\hline 
\end{tabular}
\label{tab:Robustness_PoseError}
\vspace{-3mm}
\end{table*}

\begin{table*}[!t]
\centering
\setlength\tabcolsep{2pt}
\caption{Robustness to communication latency on DAIR-V2X.}
\vspace{-3mm}
\begin{tabular}{l|ccccc}
\hline
Dataset    & \multicolumn{5}{c}{DAIR-V2X} \\ \hline
Method/Metric       &  \multicolumn{5}{c}{AP30/AP50$\uparrow$}  \\ \hline
Latency Level ($ms$)   & 0 & 100 & 200 & 300 & 500 \\ \hline
No Collaboration      & 71.35 /67.27  & 71.35 /67.27  & 71.35 /67.27  \\
Late                  & 77.37 /69.53  & 76.81 /66.74  & 72.91 /61.85  & 69.82 /60.46  & 67.11 /60.18  \\
AttFuse               & 72.39 /64.83  & 72.04 /64.03  & 70.92 /63.40  & 70.68 /63.35  & 69.50 /62.84   \\
%DiscoNet              & 82.16 /78.60  & 82.06 /77.88  & 80.94 /76.31  & 80.19 /75.15  & 78.82 /74.80  \\
V2VNet                & 83.98 /79.28  & 83.86 /77.75  & 81.65 /74.52  & 79.46 /72.51  & 76.33 /70.57  \\
Where2comm            & 84.50 /79.39  & 84.22 /77.34  & 81.46 /72.69  & 78.49 /70.62  & 74.72 /68.92  \\\hline 
\textbf{CodeFilling}  & \textbf{84.52} /\textbf{79.99}  & \textbf{84.27} /\textbf{78.34}  & \textbf{82.08} /\textbf{74.73}  & \textbf{80.10} /\textbf{72.83}  & \textbf{76.95} /\textbf{71.50} \\\hline 
\end{tabular}
\label{tab:Robustness_Latency}
\vspace{-3mm}
\end{table*}

\begin{table*}[!t]
\centering
\setlength\tabcolsep{2pt}
\caption{Robustness to communication latency on OPV2VH+.}
\vspace{-3mm}
\begin{tabular}{l|ccccc}
\hline
Dataset    & \multicolumn{5}{c}{OPV2VH+} \\ \hline
Method/Metric   &  \multicolumn{5}{c}{AP50/AP70$\uparrow$} \\ \hline
Latency Level ($ms$)   & 0 & 100 & 200 & 300 & 500  \\ \hline
No Collaboration      & 68.83 /54.27  & 68.83 /54.27  & 68.83 /54.27  & 68.83 /54.27  & 68.83 /54.27  \\
Late                  & 86.87 /79.68  & 75.85 /34.62  & 39.17 /23.91  & 32.04 /23.46  & 34.18 /26.30  \\
AttFuse               & 76.55 /53.95  & 64.90 /22.95  & 34.92 /14.38  & 24.75 /12.63  & 20.62 /12.03   \\
%DiscoNet              & 80.14 /61.13  & 69.41 /36.55  & 42.58 /22.31  & 28.61 /16.94  & 22.60 /15.07   \\
V2VNet                & 90.07 /85.73  & 83.03 /41.23  & 46.97 /18.04  & 31.56 /18.30  & 29.17 /22.68  \\
Where2comm            & 90.77 /85.53  & 83.31 /36.74  & 40.10 /14.69  & 21.73 /11.78  & 14.03 /10.00   \\\hline 
\textbf{CodeFilling}  & \textbf{90.82} /\textbf{88.19}  & \textbf{85.29} /\textbf{59.63}  & \textbf{75.16} /\textbf{58.67}  & \textbf{73.69} /\textbf{57.31}  & \textbf{71.53} /\textbf{55.84}      \\\hline 
\end{tabular}
\label{tab:Robustness_Latency}
\vspace{-3mm}
\end{table*}

\subsection{Experimental settings}

In our system, for LiDAR sensor inputs, we adopt the PointPillar detector~\cite{LangPointPillars:CVPR2018}, while for camera inputs, we follow the CaDDN~\cite{ReadingCategorical:CVPR2021}, utilizing 50 depth categories with linearly increasing spacing. To enhance learning effectiveness, we train all models in a heterogeneous setting. Consequently, in the inference phase, this model becomes versatile and applicable in homogeneous and heterogeneous settings, including camera-only, LiDAR-only, and heterogeneous setups.

For the training strategy, we initially pre-train the single-agent detector without a codebook for 30 epochs, starting with a learning rate of $2$e-$3$ and reducing it by a factor of 0.1 at the 20th epoch. This phase establishes a robust perceptual feature space. Subsequently, we train the entire collaborative perception model for 20 epochs, integrating both codebook reconstruction and perception losses. This dual supervision not only boosts learning efficiency but also ensures the codebook retains essential perceptual features, enabling a lossless performance for the perceptual task.

\section{OPV2VH+ Dataset}

\noindent
\textbf{Data generation.} We extend the original OPV2V~\cite{XuOPV2V:ICRA22} with more collaborative agents ($10$), and extend the OPV2V+~\cite{HuCollaboration:CVPR23} with more modalities. Our OPV2VH+ is co-simulated by OpenCDA~\cite{XuOpenCDA:ITSC2021} and CARLA~\cite{DosovitskiyCARLA:CoRL2017}. OpenCDA provides the driving scenarios that ensure the agents drive smoothly and safely, including the vehicle's initial location and moving speed. CARLA provides the maps, and weather and controls the movements of the agents. We replay the simulation logs of OPV2V and equip more vehicles with LiDAR, camera and depth sensors. Figure.~\ref{Fig:opv2v_single_sample} shows the LiDAR and four RGB/depth camera views (front, left, right, back) of the same agent. Figure.~\ref{Fig:OPV2VH_Sample_1} and  Figure.~\ref{Fig:OPV2VH_Sample_2} show a randomly selected data sample with 10 collaborative agents, the collected LiDAR and front view images in the same timestamp.

\begin{figure*}[!t]
    \centering
    % \hfill
    \begin{subfigure}{0.99\linewidth}
    \includegraphics[width=0.99\linewidth]{Figs/OPV2VH_Sample/1045_000068_lidar0.png}
    \caption{LiDAR}
    \hfill
  \end{subfigure}
    \begin{subfigure}{0.24\linewidth}
    \includegraphics[width=0.95\linewidth]{Figs/OPV2VH_Sample/1045_000068_camera0.png}
    \caption{Camera 0}
  \end{subfigure}
  \hfill
  \begin{subfigure}{0.24\linewidth}
    \includegraphics[width=0.95\linewidth]{Figs/OPV2VH_Sample/1045_000068_camera1.png}
    \caption{Camera 1}
  \end{subfigure}
  \hfill
  \begin{subfigure}{0.24\linewidth}
    \includegraphics[width=0.95\linewidth]{Figs/OPV2VH_Sample/1045_000068_camera2.png}
    \caption{Camera 2}
  \end{subfigure}
  \hfill
  \begin{subfigure}{0.24\linewidth}
    \includegraphics[width=0.95\linewidth]{Figs/OPV2VH_Sample/1045_000068_camera3.png}
    \caption{Camera 3}
  \end{subfigure}
  \hfill
  \begin{subfigure}{0.24\linewidth}
    \includegraphics[width=0.95\linewidth]{Figs/OPV2VH_Sample/1045_000068_depth0.png}
    \caption{Depth 0}
  \end{subfigure}
  \hfill
  \begin{subfigure}{0.24\linewidth}
    \includegraphics[width=0.95\linewidth]{Figs/OPV2VH_Sample/1045_000068_depth1.png}
    \caption{Depth 1}
  \end{subfigure}
  \hfill
  \begin{subfigure}{0.24\linewidth}
    \includegraphics[width=0.95\linewidth]{Figs/OPV2VH_Sample/1045_000068_depth2.png}
    \caption{Depth 2}
  \end{subfigure}
  \hfill
  \begin{subfigure}{0.24\linewidth}
    \includegraphics[width=0.95\linewidth]{Figs/OPV2VH_Sample/1045_000068_depth3.png}
    \caption{Depth 3}
  \end{subfigure}
  \vspace{-2mm}
  \caption{Each agent is equipped with 1 LiDAR, 4 cameras, and 4 depth sensors in OPV2VH+.}
  \label{Fig:opv2v_single_sample}
  \vspace{-2mm}
\end{figure*}

\begin{figure*}[!t]
  \centering
  \hfill
  \begin{subfigure}{0.55\linewidth}
    \includegraphics[width=0.99\linewidth]{Figs/OPV2VH_Sample/1045_000068_lidar0.png}
    \caption{Agent 0: LiDAR 0}
  \end{subfigure}
  \begin{subfigure}{0.21\linewidth}
    \includegraphics[width=0.99\linewidth]{Figs/OPV2VH_Sample/1045_000068_camera0.png}
    \caption{Agent 0: Camera 0}
  \end{subfigure}
  \hfill
  \begin{subfigure}{0.21\linewidth}
    \includegraphics[width=0.99\linewidth]{Figs/OPV2VH_Sample/1045_000068_depth0.png}
    \caption{Agent 0: Depth 0}
  \end{subfigure}
  \hfill
  \begin{subfigure}{0.55\linewidth}
    \includegraphics[width=0.99\linewidth]{Figs/OPV2VH_Sample/1054_000068_lidar0.png}
    \caption{Agent 1: LiDAR 0}
  \end{subfigure}
  \hfill
  \begin{subfigure}{0.21\linewidth}
    \includegraphics[width=0.99\linewidth]{Figs/OPV2VH_Sample/1054_000068_camera0.png}
    \caption{Agent 1: Camera 0}
  \end{subfigure}
  \hfill
  \begin{subfigure}{0.21\linewidth}
    \includegraphics[width=0.99\linewidth]{Figs/OPV2VH_Sample/1054_000068_depth0.png}
    \caption{Agent 1: Depth 0}
  \end{subfigure}
  \hfill
  \begin{subfigure}{0.55\linewidth}
    \includegraphics[width=0.99\linewidth]{Figs/OPV2VH_Sample/1067_000068_lidar0.png}
    \caption{Agent 2: LiDAR 0}
  \end{subfigure}
  \hfill
  \begin{subfigure}{0.21\linewidth}
    \includegraphics[width=0.99\linewidth]{Figs/OPV2VH_Sample/1067_000068_camera0.png}
    \caption{Agent 2: Camera 0}
  \end{subfigure}
  \hfill
  \begin{subfigure}{0.21\linewidth}
    \includegraphics[width=0.99\linewidth]{Figs/OPV2VH_Sample/1067_000068_depth0.png}
    \caption{Agent 2: Depth 0}
  \end{subfigure}
  \hfill
  \begin{subfigure}{0.55\linewidth}
    \includegraphics[width=0.99\linewidth]{Figs/OPV2VH_Sample/1068_000068_lidar0.png}
    \caption{Agent 3: LiDAR 0}
  \end{subfigure}
  \hfill
  \begin{subfigure}{0.21\linewidth}
    \includegraphics[width=0.99\linewidth]{Figs/OPV2VH_Sample/1068_000068_camera0.png}
    \caption{Agent 3: Camera 0}
  \end{subfigure}
  \hfill
  \begin{subfigure}{0.21\linewidth}
    \includegraphics[width=0.99\linewidth]{Figs/OPV2VH_Sample/1068_000068_depth0.png}
    \caption{Agent 3: Depth 0}
  \end{subfigure}
  \hfill
  \begin{subfigure}{0.55\linewidth}
    \includegraphics[width=0.99\linewidth]{Figs/OPV2VH_Sample/1070_000068_lidar0.png}
    \caption{Agent 4: LiDAR 0}
  \end{subfigure}
  \hfill
  \begin{subfigure}{0.21\linewidth}
    \includegraphics[width=0.99\linewidth]{Figs/OPV2VH_Sample/1070_000068_camera0.png}
    \caption{Agent 4: Camera 0}
  \end{subfigure}
  \hfill
  \begin{subfigure}{0.21\linewidth}
    \includegraphics[width=0.99\linewidth]{Figs/OPV2VH_Sample/1070_000068_depth0.png}
    \caption{Agent 4: Depth 0}
  \end{subfigure}
  \vspace{-2mm}
  \caption{Agents 0 through 4 in a data sample comprising 10 agents from the OPV2VH+ dataset.}
  \label{Fig:OPV2VH_Sample_1}
  \vspace{-2mm}
\end{figure*}

\begin{figure*}[!t]
  \centering
  \hfill
  \begin{subfigure}{0.55\linewidth}
    \includegraphics[width=0.99\linewidth]{Figs/OPV2VH_Sample/1071_000068_lidar0.png}
    \caption{Agent 5: LiDAR 0}
  \end{subfigure}
  \hfill
  \begin{subfigure}{0.21\linewidth}
    \includegraphics[width=0.99\linewidth]{Figs/OPV2VH_Sample/1071_000068_camera0.png}
    \caption{Agent 5: Camera 0}
  \end{subfigure}
  \hfill
  \begin{subfigure}{0.21\linewidth}
    \includegraphics[width=0.99\linewidth]{Figs/OPV2VH_Sample/1071_000068_depth0.png}
    \caption{Agent 5: Depth 0}
  \end{subfigure}
  \hfill
  \begin{subfigure}{0.55\linewidth}
    \includegraphics[width=0.99\linewidth]{Figs/OPV2VH_Sample/1072_000068_lidar0.png}
    \caption{Agent 6: LiDAR 0}
  \end{subfigure}
  \hfill
  \begin{subfigure}{0.21\linewidth}
    \includegraphics[width=0.99\linewidth]{Figs/OPV2VH_Sample/1072_000068_camera0.png}
    \caption{Agent 6: Camera 0}
  \end{subfigure}
  \hfill
  \begin{subfigure}{0.21\linewidth}
    \includegraphics[width=0.99\linewidth]{Figs/OPV2VH_Sample/1072_000068_depth0.png}
    \caption{Agent 6: Depth 0}
  \end{subfigure}
  \hfill
  \begin{subfigure}{0.55\linewidth}
    \includegraphics[width=0.99\linewidth]{Figs/OPV2VH_Sample/1073_000068_lidar0.png}
    \caption{Agent 7: LiDAR 0}
  \end{subfigure}
  \hfill
  \begin{subfigure}{0.21\linewidth}
    \includegraphics[width=0.99\linewidth]{Figs/OPV2VH_Sample/1073_000068_camera0.png}
    \caption{Agent 7: Camera 0}
  \end{subfigure}
  \hfill
  \begin{subfigure}{0.21\linewidth}
    \includegraphics[width=0.99\linewidth]{Figs/OPV2VH_Sample/1073_000068_depth0.png}
    \caption{Agent 7: Depth 0}
  \end{subfigure}
  \hfill
  \begin{subfigure}{0.55\linewidth}
    \includegraphics[width=0.99\linewidth]{Figs/OPV2VH_Sample/1077_000068_lidar0.png}
    \caption{Agent 8: LiDAR 0}
  \end{subfigure}
  \hfill
  \begin{subfigure}{0.21\linewidth}
    \includegraphics[width=0.99\linewidth]{Figs/OPV2VH_Sample/1077_000068_camera0.png}
    \caption{Agent 8: Camera 0}
  \end{subfigure}
  \hfill
  \begin{subfigure}{0.21\linewidth}
    \includegraphics[width=0.99\linewidth]{Figs/OPV2VH_Sample/1077_000068_depth0.png}
    \caption{Agent 8: Depth 0}
  \end{subfigure}
  \hfill
  \begin{subfigure}{0.55\linewidth}
    \includegraphics[width=0.99\linewidth]{Figs/OPV2VH_Sample/1080_000068_lidar0.png}
    \caption{Agent 9: LiDAR 0}
  \end{subfigure}
  \hfill
  \begin{subfigure}{0.21\linewidth}
    \includegraphics[width=0.99\linewidth]{Figs/OPV2VH_Sample/1080_000068_camera0.png}
    \caption{Agent 9: Camera 0}
  \end{subfigure}
  \hfill
  \begin{subfigure}{0.21\linewidth}
    \includegraphics[width=0.99\linewidth]{Figs/OPV2VH_Sample/1080_000068_depth0.png}
    \caption{Agent 9: Depth 0}
  \end{subfigure}
  \vspace{-2mm}
  \caption{Agents 5 through 9 in a data sample comprising 10 agents from the OPV2VH+ dataset.}
  \label{Fig:OPV2VH_Sample_2}
  \vspace{-2mm}
\end{figure*}

\noindent
\textbf{Data collection.} We collect synchronous images from all 4 cameras, 4 depth sensors, and 1 LiDAR sensor on all the collaborative vehicles in a sample. LiDAR extrinsic, camera/depth sensor intrinsics, and extrinsic in global coordinates are provided to support coordinate transformation across various collaborative vehicles. During data collection, 3D bounding boxes of vehicles in the scene are recorded at the same moment with sensor inputs, including location (x, y, z), rotation (w, x, y, z in quaternion) in the global coordinate, and their length, width, and height. The location (x, y, z) is the center of the bounding box. In total, 10,416 samples, 10,4160 point cloud sweeps, 416,640 RGB/depth images, and 482,037 3D bounding boxes are collected.

\textbf{Data usage.} We randomly split the samples into train/validation/test, resulting 6736/1980/1700 samples, 67,360/19,800/17,000 LiDAR sweeps, 269,400/79,200/68,000 images, and 333,543/75,289/73,205 3D bounding boxes. The dataset is organized in a similar way to the OPV2V~\cite{XuOPV2V:ICRA22} and OPV2V+~\cite{HuCollaboration:CVPR23} dataset; so it can be used directly with the original dataset processing tool-kits.

\section{Benchmarks}
We conduct extensive experiments on all two widely used collaborative perception benchmarks covering three types of collaboration settings: i) all the collaborative agents use cameras, ii) all the collaborative agents use LiDARs, and iii) the collaborative agents randomly use camera or LiDAR. Regarding the heterogeneous setup, agents are randomly assigned either LiDAR or camera, resulting in a balanced 1:1 ratio of agents across the different modalities.

Tab.~\ref{tab:SOTA_performance} presents the overall performance on the real-world dataset, DAIR-V2X~\cite{YuDAIRV2X:CVPR22}, and the extended simulation dataset OPV2VH+. We see that \texttt{CodeFilling} consistently achieves significant improvements over previous methods on all the benchmarks.

Tab.~\ref{tab:Robustness_PoseError} and Tab.~\ref{tab:Robustness_Latency} presents the overall performance under realistic issues on the real-world dataset, DAIR-V2X~\cite{YuDAIRV2X:CVPR22}, and the extended simulation dataset OPV2VH+. We see that \texttt{CodeFilling} is more robust to the pose error and communication latency issues.
